# Supplementary material for: A Perceptual Measure for Evaluating the Resynthesis of Automatic Music Transcriptions
Source: arXiv:2202.12257 source file (2022-03-07)
Supplement: Supplementary file 1 [file supplementary01.pdf]

# A Perceptual Measure for Resynthesis of AMT

Supplementary Materials

Federico Simonetta, Federico Avanzini, Stavros Ntalampiras

February 24, 2022

## 1 SI Model

SI is based on a previous work [3], that, to our knowledge, is the only one that predicts both alignment and midi velocities. The inputs are a non-aligned score and an audio recording, while the output is a list of midi notes each associated with onsets, offsets and velocity.

For the alignment stage, the original work use an innovative method. Usually, audio-to-score alignment methods convert audio and score to a common representation to exploit *Dynamic Time Warping* (DTW) for the alignment. The most used and effective approach consisted in synthesizing the music score into audio, so that DTW could be performed in the audio domain [1]. The innovation of the method is to translate the audio recording to a pianoroll representation using a piano AMT system; the result is a much more precise alignment [4]. Piano-rolls are 2D boolean matrices with $K$ rows and $N$ columns; the entry $(k, n)$ represents the state of pitch $k$ at time $n$. Usually, $K$ is set to 128 so that it is in direct relationship with MIDI specifications. The two pianorolls, one from the audio and one from the score, can then be aligned using DTW. This will create a mapping between columns (frames) in the score domain and columns in the audio domain, which can be used to recompute the correct duration of the notes in score without relying on the AMT output, which is prone to errors in pitch identification.

Following the same approach, we used the new O&F model for the alignment, which by itself has a greater precision than the method previously used. The second improvement we made is the use of 3-valued pianorolls: we introduced a new value to represent the onset of a note. This increased the precision of the successive DTW because repeated notes are often not distinguishable in the boolean pianoroll if the onset is immediately after the offset of the previous note. Moreover, the introduction of a new value works as "anchor" for the DTW algorithm, which tries to find correspondences between the alternations of three values instead of only two. The third improvement we made was to finely realign the aligned score by realigning short excerpts similarly to [2]. Namely, after the first alignment, we further perform the DTW between windows of the previously realigned score and the corresponding windows of the transcribed

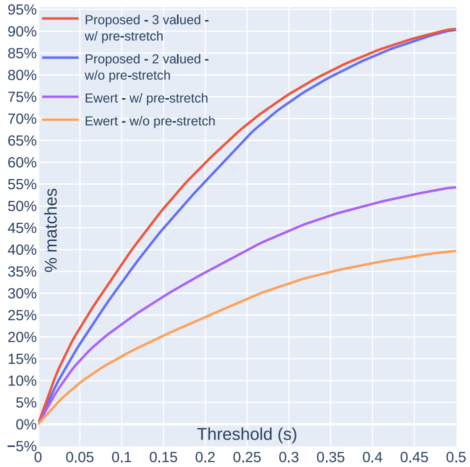


Figure 1: Our proposed alignment method compared to a famous baseline [1] (Ewert). "% matches" are the percentage of notes for which both onset and offset are aligned with an error less than the given threshold

pianoroll. We repeated this steps 3 times with windows lasting 10, 5 and 1 seconds with 50% of overlap. Finally, we pre-stretched the misaligned score so that the number of columns corresponded to the number of frames in the transcription; we used 0.001 seconds per column. Results are shown in figure 1, where we use the *SMD* [6] dataset provided by *ASMD* [8] to compare a de facto standard baseline [1] with our method with and without pre-stretching and with 2-valued or 3-valued pianoroll. We empirically found that FastDTW [7] is much more efficient with no loss of efficacy in respect to pure DTW; we treated the distance function and the radius as hyper-parameters and tuned them using the MIDI data of the piano pieces in the MusicNet dataset [9], selected thanks to *ASMD*, which also provides misaligned data. Results showed that cosine distance with radius of 10 were the best performing parameters for FastDTW on midi-to-midi alignment.

After having aligned the score, the original method performs a note velocity estimation using Non-negative Matrix Factorization (NMF): first, they build an initial template by analyzing the sound produced by a virtual instrument, building a multi-basis model that separates the template of the various parts of the note – i.e. the spectrum of the onset is supposed to be different from the one of the decay and of the release; second, they use the aligned pianoroll to initialize the activation; third, they run the NMF optimization and use the produced template and activation to compute mini-spectrograms for each note. They can finally use these mini-spectrograms as input of feed-forward neural network for predicting the velocity.

We followed the same approach but with few modifications. First, we used a CQT-based spectrogram which eases the comparison with the pianoroll [5].

Secondly, we empirically found that using CQT instead of FFT, the usual SGD optimization was enough and that the constraints added in the original work produced no visible modification in the output spectrogram. We used longer frames lasting 16384 samples with 22050 Hz as sampling rate and 1024 samples as hop size; we used 20 basis instead of 10: each pitch is thus modeled with 20 different templates according to the duration of the note. The initial templates for each basis of each pitch were built averaging the corresponding frames from a MIDI synthesized with the free *Salamander Grand Piano*[1]; the MIDI contained all the 88 piano notes played with 10 different velocity layers, 2 different duration (0.1 and 1.5 seconds), and 3 inter-notes types of silence (0 seconds, 1 seconds and a slight overlap of 0.02 seconds). Instead of using 0 values in the initial activation, we use a default value of 1e-4; this should allow the optimization to align the activation even more finely while still using the multiplicative updates as in the original work. We run 5 iterations of NMF and then other 5 without updating the templates. Then, for each note we look for the maximum value in the activation, which is tied to the onset time; we chose 14 columns around that point and use the templates of that pitch to compute the mini-spectrogram. Our neural network takes as input the flattened mini-spectrogram and passes it through 16 different branches, each made by a fully connected layer with learnt bias and the SELU activation function. Each branch should take care of 8 different velocities and thus outputs 9 values: 8 for estimating the probability of each velocity value and 1 for estimating the probability that the velocity is in that branch; this last value is thus passed into a softmax function so that the sum of the probability of being in a branch is 1. All the outputs from all the branches are then passed through 5 fully connected layers with SELU activation and no bias and then a fully connected layer with only one output and sigmoid activation. The output is then multiplied by 128 and rounded to the nearest integer. During training we used L1 loss against the output velocity estimation and Binary Cross Entropy against the estimated probability for each branch. We also used early-stop of 10 epochs and batch size of 400. The dataset consisted of 100 random songs from the Maestro dataset [2], with misaligned scores as provided by *ASMD*; from them, we extracted 474 429 mini-spectrograms as described earlier and separated them into training, validation and test set with 70-15-15 proportion, resulting in 831 batches in train and 178 in test and validation sets. We obtained an average error of 15.11 with standard deviation of 10.94 for the test set, using 251 epochs after which the early-stop algorithm terminated the training.

# References


[1] Sebastian Ewert, Meinard Muller, and Peter Grosche. High resolution audio synchronization using chroma onset features. *ICASSP*, 2009.


[1] free as in speech: https://musical-artifacts.com/artifacts/533

[2] Curtis Hawthorne, Andriy Stasyuk, Adam Roberts, Ian Simon, Cheng-Zhi Anna Huang, Sander Dieleman, Erich Elsen, Jesse H. Engel, and Douglas Eck. Enabling factorized piano music modeling and generation with the maestro dataset. *ICLR*, 2019.

[3] Dasaem Jeong, Taegyun Kwon, and Juhan Nam. Note-intensity estimation of piano recordings using coarsely aligned midi score. *JAES*, 68, 2020.

[4] Taegyun Kwon, Dasaem Jeong, and Juhan Nam. Audio-to-score alignment of piano music using rnn-based automatic music transcription. *SMC*, 2017.

[5] Meinard Müller. *Fundamentals of Music Processing: Audio, Analysis, Algorithms, Applications*. 1 edition, 2015.

[6] Meinard Müller, Verena Konz, Wolfgang Bogler, and Vlora Arifi-Müller. Saarland music data (smd). *ISMIR*, 2011.

[7] Stan Salvador and Philip Chan. Toward accurate dynamic time warping in linear time and space. *Intelligent Data Analysis*, 2007.

[8] Federico Simonetta, Stavros Ntalampiras, and Federico Avanzini. Asmd: an automatic framework for compiling multimodal datasets. *SMC*, 2020.

[9] John Thickstun, Zaïd Harchaoui, Dean P. Foster, and Sham M. Kakade. Invariances and data augmentation for supervised music transcription. *ICASSP*, 2018.
